# Supplementary material for: Toward a Better Understanding of Loss Functions for Collaborative Filtering
Source: arXiv:2308.06091 source file (2023-10-30)
Supplement: Supplementary file 1 [file sec-appendix__backup_.tex]

\newpage

\appendix

\input{Tables/exp-table-pop_unpop_user_acc}


\section{Minimization of Margin-aware Alignment Loss Function}
우리는 $M_{ui}$를 $M_u$와 $M_i$의 합으로 표현하는 MA loss function이 BC~\cite{ZhangMWC22}보다 더 user/item-specific한 임베딩을 학습할 수 있다는 것을 이론적으로 증명한다.

\begin{theorem} \label{minimization_ma}
    Assuming the user and item embeddings are normalized, the minimization of MA loss function is equivalent to minimizing a compactness part. The compactness part makes user/item embeddings closer to the averaged item/user embeddings that reflect user/item-specific information (\eg, user/item popularitiess).
\end{theorem}
\begin{align}
\mathcal{L}_{M A} \stackrel{\mathrm{c}}{=} \sum_{u \in \mathcal{U}}\left\|v_u-R_u^{\normalfont \text{T}} c_u^R\right\|^2+\sum_{i \in \mathcal{I}}\left\|v_i-R_i^{\normalfont \text{T}} c_i^R\right\|^2,
\end{align}
where $\stackrel{\mathrm{c}}{=}$ denotes equality up to multiplicative or additive constant. $c_u^R=\frac{1}{\left|\mathcal{P}_u\right|} \sum_{i \in \mathcal{P}_u} R_i v_i$ and $c_i^R=\frac{1}{\left|\mathcal{P}_i\right|} \sum_{u \in \mathcal{P}_i} R_u v_u$ denote average of rotated item and user embeddings, respectively. $\mathcal{P}_u$ and $\mathcal{P}_i$ are a set of items by user $u$ and a set of users by item $i$, respectively. $R_u$ and $R_i$ are rotation matrices of user and item embeddings with the margins $M_u$ and $M_i$, respectively. Besides, $v_u$ and $v_i$ are L2-normalized user and item embedding, respectively~\footnote{For visibility of formulas, we denote $v_u$ and $v_i$ instead of $\Tilde{f(u)}$ and $\Tilde{f(i)}$, respectively.}.


\begin{proof} \label{proof_minimization_ma}
Theorem~\ref{minimization_ma}를 증명하기 위해, 우리는 BC~\cite{ZhangMWC22}의 theoretical property로부터 영감을 받았다. 이 theoretical property는 BC를 최소화하면, compactness와 dispersion 두 가지 부분을 동시에 최적화하는 의미를 가진다.

\begin{align}\label{eq:minimization_bc}
    \mathcal{L}_{BC} \geq \sum_{u \in \mathcal{U}}\left\|v_u-c_u\right\|^2+\sum_{i \in \mathcal{I}}\left\|v_i-c_i\right\|^2-\sum_{u \in \mathcal{U}} \sum_{j \in \mathcal{N}_u}\left\|v_u-c_j\right\|^2,
\end{align}
where $c_u=\frac{1}{\left|\mathcal{P}_u\right|} \sum_{i \in \mathcal{P}_u} v_i$ and $c_i=\frac{1}{\left|\mathcal{P}_i\right|} \sum_{u \in \mathcal{P}_i} v_u$ denote averaged item and user embeddings, respectively.


첫 번째 부분은 i) compactness로 사용자 임베딩을 항목 임베딩의 평균과 가깝게 만들어주는 부분이고 (\ie, 앞의 두 항), 두 번째 부분은 ii) dispersion으로 사용자와 항목 간의 거리를 멀게 만들어주는 부분 (\ie, 마지막 항)이다. 두 번째 부분인 dispersion은 uniformity를 의미하며 WU loss function과 대응되는 개념이기 때문에, 우리는 첫 번째 부분 compactness를 참고하여 MA loss function의 compactness를 증명하는 것을 목표로 한다.

사용자/항목 마진 (\ie, $M_u$ and $M_i$)만큼 사용자/항목 임베딩을 회전시키는 회전 행렬 (\ie, $R_u$ and $R_i$)이 존재한다고 가정하면, MA loss는 다음과 같이 표현된다.
\begin{align}
    \mathcal{L}_{MA}=-\sum_{(u, i) \in \mathcal{D}}\cos \left(\hat{\theta}_{ui}+M_u+M_i\right)=-\sum_{(u, i) \in \mathcal{D}}\left(R_u v_u\right)^{\text{T}}\left(R_i v_i\right).
\end{align}

여기서, $v_u$와 $v_i$는 unit vectors (\ie, $v_u^T v_i=1-\frac{1}{2}\left\|v_u-v_i\right\|^2$)임을 활용해 전개하면 다음과 같다.

\begin{align}
& -\sum_{(u, i) \in \mathcal{D}}\left(R_u v_u\right)^{\text{T}}\left(R_i v_i\right) \stackrel{\mathrm{c}}{=} \sum_{(u, i) \in \mathcal{D}}\left\|R_u v_u-R_i v_i\right\|^2 \\
& =\sum_{u \in \mathcal{U}} \sum_{i \in \mathcal{P}_u}\left(\left\|R_u v_u\right\|^2-v_u^{\text{T}} R_u^{\text{T}} R_i v_i\right)+\sum_{i \in \mathcal{I}} \sum_{u \in \mathcal{P}_i}\left(\left\|R_i v_i\right\|^2-v_u^{\text{T}} R_u^{\text{T}} R_i v_i\right) \\
& =\sum_{u \in \mathcal{U}}\left(\left|\mathcal{P}_u\right| v_u^{\text{T}} R_u^{\text{T}} R_u v_u-v_u^{\text{T}} R_u^{\text{T}} \sum_{i \in \mathcal{P}_u} R_i v_i\right) \nonumber \\
& \qquad\qquad\qquad + \sum_{i \in \mathcal{I}}\left(\left|\mathcal{P}_i\right| v_i^{\text{T}} R_i^{\text{T}} R_i v_i-v_i^{\text{T}} R_i^{\text{T}} \sum_{u \in \mathcal{P}_i} R_u v_u\right) \\
& =\sum_{u \in \mathcal{U}}\left(\left|\mathcal{P}_u\right| v_u^{\text{T}}\left(v_u-\frac{R_u^{\text{T}}}{\left|\mathcal{P}_u\right|} \sum_{i \in \mathcal{P}_u} R_i v_i\right)\right) \nonumber \\
& \qquad\qquad\qquad + \sum_{i \in \mathcal{I}}\left(\left|\mathcal{P}_i\right| v_i^{\text{T}}\left(v_i-\frac{R_i^{\text{T}}}{\left|\mathcal{P}_i\right|} \sum_{u \in \mathcal{P}_i} R_u v_u\right)\right) \\
& =\sum_{u \in \mathcal{U}}\left(\left|\mathcal{P}_u\right| v_u^{\text{T}}\left(v_u-R_u^{\text{T}} c_u^R\right)\right) + \sum_{i \in \mathcal{I}}\left(\left|\mathcal{P}_i\right| v_i^{\text{T}}\left(v_i-R_i^{\text{T}} c_i^R\right)\right) \\
& \stackrel{\mathrm{c}}{=} \sum_{u \in \mathcal{U}}\left\|v_u-R_u^{\text{T}} c_u^R\right\|^2+\sum_{i \in \mathcal{I}}\left\|v_i-R_i^{\text{T}} c_i^R\right\|^2. \label{proof_final}
\end{align}


결과적으로, Eq~\eqref{proof_final}로부터 MA loss function은 사용자 임베딩을 user-specific 정보 (\eg, user popularity)를 반영한 항목 임베딩의 평균에 가깝게 만드는 것을 확인할 수 있다 (and vice versa). 이는 단순히 사용자 임베딩을 항목 임베딩의 평균에 가깝게 만드는 것 (\ie, BC~\cite{ZhangMWC22})에 비해 user-specific 정보를 반영할 수 있기 때문에, MA loss function이 더 의미있는 임베딩을 얻을 수 있다는 것을 보여준다. % 또한, MA loss function은 $c_u^R$을 계산할 때 회전시킨 항목 임베딩을 사용하기 때문에, 항목 마진도 고려한다. 다시 말해, 사용자 임베딩을 학습할 때 사용자와 항목 마진을 모두 고려한다 (and vice versa).

\end{proof}

\section{Performance analysis by user popularity}
MAWU의 성능 향상이 어디서 왔는지 분석하기 위해, user popularity 기준으로 2:8로 user group을 나눠 성능을 확인한다. Table~\ref{tab:pop_unpop_user_acc}는 MAWU가 DirectAU~\cite{WangYMZCLM22}에 비해 두 group에서 성능 향상이 있음을 보여준다. 이는 데이터셋의 특성에 따라 달라지는 것으로 보인다.


\section{Related Work on Various Loss Functions in Collaborative Filtering}
%%% CF loss 연구 동향 요약
\textbf{Overview.} 추천 시스템에서 많이 사용해왔던 전통적인 loss로는 MSE, BCE~\cite{HuKV08}, and BPR~\cite{RendleFGS09}을 들 수 있다. 아직까지도 많은 SOTA 모델들이 이 loss들을 즐겨 사용함과 동시에 최근 CF에서 다양한 loss function들~\cite{HsiehYCLBE17, LiZZQZHH20, GaoCPSV22, MaoZWDDXH21, WuWGCFQH22, WangYMZCLM22, ZhuoZYZ22}이 제안되고 있다. 단순히 loss만 변경했을 뿐인데 SOTA 모델들을 뛰어넘는 성능을 보여주면서~\cite{MaoZWDDXH21, WuWGCFQH22, GaoCPSV22, WangYMZCLM22}, 해당 연구들이 더욱 주목을 끌고 있다. CF loss 연구의 흐름을 살펴보면, metric learning~\cite{HsiehYCLBE17, LiZZQZHH20}부터 contrastive learning~\cite{WuWF0CLX21, YuY00CN22, WuWGCFQH22, ZhangMWC22}까지 representation learning 관점에서 발전해왔다. 최근에는 contrastive loss를 alignment와 uniformity로 표현한 loss가 높은 성능을 보여주고 있다~\cite{WangYMZCLM22}. 또한, 성능을 boosting할 수 있는 module-type loss~\cite{GaoCPSV22, ZhuoZYZ22}나 hyperbolic space에서 representation learning을 하는 loss~\cite{0001L00K22, 000100LK22}가 제안되고 있다.

%%% metric learning 관련 loss (CML, SML)
\vspace{1mm}
\noindent
\textbf{Metric learning.}
\citet{HsiehYCLBE17}이 metric learning 개념을 CF에 처음 도입함으로써 loss function 개발의 포문을 열었다. CML~\cite{HsiehYCLBE17}은 user와 positive item과의 거리가 user와 negative item과의 거리보다 짧아져야 된다는 직관적인 개념을 loss에 녹아냈다. CML은 user를 중심으로 items와의 관계 (\ie, user-centric loss)만을 활용했다면, \citet{LiZZQZHH20}에서는 item-centric loss 개념을 추가한다. 또한, margin을 constant로 둔 CML과 달리 SML~\cite{LiZZQZHH20}은 margin을 adaptively 학습한다.

%%% contrastive learning 관련 loss (CCL, SSM, BC Loss)
\vspace{1mm}
\noindent
\textbf{Contrastive learning.}
이후, contrastive learning 관점으로 해석되는 loss function들~\cite{MaoZWDDXH21, WuWF0CLX21, ZhouMZZY21, YuY00CN22, WuWGCFQH22, ZhangMWC22}이 제안되었다. 단순한 형태의 contrastive loss인 CCL~\cite{MaoZWDDXH21}은 MSE와 비슷한 형태를 가지며, constant margin을 통해 hard negative sampling을 한다. 다음으로, 다른 도메인 (\eg, computer vision and natual language processing)에서 많이 사용하는 contrastive loss인 InfoNCE~\cite{abs-1807-03748} and NT-Xent~\cite{ChenK0H20} loss를 추천 시스템에서도 활용하고 있다~\cite{WuWF0CLX21, ZhouMZZY21, YuY00CN22, WuWGCFQH22, ZhangMWC22}. 특히, \citet{WuWGCFQH22}는 이러한 형태가 popularity bias를 완화하고, hard negative sampling 효과를 가진다는 것을 증명하여 추천 시스템과의 적합성을 보여준다. 이와 같은 증명에 힘입어, \citet{ZhangMWC22}는 SSM~\cite{WuWGCFQH22}에 angular margin을 추가한 loss를 제시한다. 이 margin은 user와 positive item의 popularity embedding이 이루는 각도만큼 user embedding이 학습될 수 있는 공간을 제한한다.

%%% alignment and uniformity 관련 loss (DirectAU)
\vspace{1mm}
\noindent
\textbf{Alignment and uniformity.}
최근, contrastive loss를 새로운 두 가지 properties로 해석하는 시도들~\cite{WangI20, WangYMZCLM22}이 나타나고 있다. \citet{WangI20}에서는 contrastive loss를 최소화하면, alignment와 uniformity를 최적화하는 것과 동일한 효과를 가진다는 것을 수식적으로 증명한다. 이 증명에 영감을 받아 \citet{WangYMZCLM22}는 BPR loss가 perfect alignment and uniformity 조건을 가질 때, vanilla BPR loss보다 작은 값을 가진다는 것을 이끌어 냈다. 이를 기반으로, \citet{WangYMZCLM22}에서는 처음으로 CF에서 alignment와 uniformity를 직접 최적화하는 DirectAU~\cite{WangYMZCLM22}를 제안했다. % 본 논문에서는, DirectAU처럼 alignment와 uniformity를 직접 최적화한다. % DirectAU는 negative sampling을 하지 않아도 된다는 큰 이점이 있다.

%%% module-type losses (MCL, UIB)
\vspace{1mm}
\noindent
\textbf{Modularization.}
기존 loss function을에 덧붙일 수 있는 module형 loss~\cite{GaoCPSV22, ZhuoZYZ22}가 제안되었다. 구체적으로, MCL~\cite{GaoCPSV22}은 BPR과 triplet loss의 weight analysis를 기반으로 loss에 여러 weighting parameter를 추가한다. \citet{ZhuoZYZ22}은 기존의 fixed boundary가 아닌 flexible boundary를 도입한다. flexible boundary를 user interest boundary로 여기고, 해당 boundary를 기준으로 positive score와 negative score를 나눈다.

%%% hyperbolic space (HRCF, HICF)
\vspace{1mm}
\noindent
\textbf{Hyperbolic space.}
앞선 loss function을들은 모두 Euclidean space에서 연산을 수행한 반면에, \citet{000100LK22}는 hyperbolic space에서 distance를 계산해 triplet margin loss를 사용한다. hyperbolic space의 기하학적 특성은 모델에 풍부한 정보를 제공한다. HICF~\cite{0001L00K22}는 HRCF~\cite{000100LK22}에 hyperbolic space 관점에서 margin learning strategy와 negative sampling method를 개선한다.

%%% loss 관련 다른 시도들 (loss search, generation, and customization)
\vspace{1mm}
\noindent
\textbf{Others.}
하나의 loss function을 설계하는 것뿐만 아니라, loss function search~\cite{LiYLGWYO19, WangWCZ020}나 loss function의 optimization scheduling 하는 연구~\cite{XuZHLSX19}도 활발히 진행되고 있다. 이와 같은 연구의 영향을 받아, 추천 시스템에서도 auto machine learning을 활용해 loss를 generation하거나 loss를 customize하는 연구~\cite{ZhaoLFLTW21, LiJGZ22, TangBLLZ22}들이 이루어지고 있다. 이러한 흐름에 발맞춰, 본 연구는 development of CF loss functions에서의 milestone이 되고자 한다.


\section{Discussion}
% \subsection{Relationships among Pointwise Loss Functions}
% 앞서 언급했듯이, pointwise loss functions은 pairwise/setwise loss functions과 수식적으로 연결되지 않는다. 하지만, pointwise loss functions (\ie, BCE, MCL, and UIB) 간은 다음과 같이 수식적으로 연결될 수 있다.

\subsection{Recent Graph Contrastive Learning-based Models}
최근 Graph Contrastive Learning (GCL) 기반 모델들이 높은 성능을 보이며 효과성을 입증하고 있다~\cite{WuWF0CLX21, YuY00CN22, CaiHXR23}. 그래서 우리는 GCL 기반 모델들과 전통 모델의 loss function과의 수식적인 차이를 확인한다. 엄밀하게, 대부분의 GCL 기반 모델들은 recommendation loss와 contrastive loss 두 가지 term으로 구성된 loss를 사용하고 있다. (\ie, $\mathcal{L}_{GCL} = \mathcal{L}_{Rec} + \lambda \mathcal{L}_{CL}$) 여기서, 첫 번째 loss인 recommendation loss $\mathcal{L}_{Rec}$는 추천 시스템에서 기본적으로 사용하는 loss다. $\mathcal{L}_{Rec}$에는 $\mathcal{L}_{Pointwise}$, $\mathcal{L}_{Pairwise}$, $\mathcal{L}_{Setwise}$, and $\mathcal{L}_{AU}$가 들어간다고 볼 수 있다. 다시 말해, 기존 loss에 GCL 기반 모델들이 사용하는 loss $\mathcal{L}_{CL}$를 추가적으로 활용하여 성능 향상을 기대해볼 수 있다. \cite{WuWF0CLX21, YuY00CN22, CaiHXR23}에서는 모두 $\mathcal{L}_{Rec}$로써 BPR을 사용한다. 그리고 두 번째 contrastive loss $\mathcal{L}_{CL}$은 user와 item을 각각 2개의 view로 augmentation하여 augmented user와 item에 대해 contrastive learning을 실시한다. (\ie, $\mathcal{L}_{CL} = \mathcal{L}_{CL-user} + \mathcal{L}_{CL-item}$) $\mathcal{L}_{CL}$를 계산할 때, 어떤 augmentation을 설계하느냐에 따라 GCL 기반 모델들은 구분된다. SGL~\cite{WuWF0CLX21}은 node/edge dropout을 한 graph augmentation을 사용하고, SimGCL~\cite{YuY00CN22}은 random noise를 직접 부여한 user/item embedding을 augmentation으로 활용한다. 또한, LightGCL~\cite{CaiHXR23}은 adjacency matrix 위에서 SVD를 수행하고, 이를 통해 얻은 recontructed graph를 augmentation으로 사용한다.


% \subsection{Designing Loss Functions in the Future}
% 이 섹션에서는 앞으로의 loss function 연구에 대한 message를 전달하고자 한다. 본 논문에서는 BC가 제일 일반화된 방식이라고 소개하고 있지만, BC가 무조건 옳은 방식은 아니고 다른 방식이 더 좋을 수 있다. 하지만, 앞으로 CF loss function를 설계함에 있어 본 논문에서 진행한 분석을 참고하면 유용할 것이다. 생각해보면 좋을 고민 한 가지를 남겨두려고 한다. DirectAU가 negative sampling을 사용하지 않아도 되는 것은 장점이지만, 반대로 유용한 negative sampling을 사용할 수 없다는 것은 단점으로 볼 수 있다. 이러한 점을 고려하여 본인의 상황과 환경에 맞게 loss function를 설계하는 것이 필요하다.
